# Supplementary material for: Quantum Monte Carlo Calculation of the Binding Energy of Bilayer Graphene
Source: arXiv:1506.08920 ancillary file (2015-06-30)
Supplement: Supplementary file 1 [file supplemental.pdf]

# Quantum Monte Carlo Calculation of the Binding Energy of Bilayer Graphene: Supplemental Material

E. Mostaani, N. D. Drummond, and V. I. Fal'ko
*Department of Physics, Lancaster University, Lancaster LA1 4YB, United Kingdom*

## I. ATOMIZATION ENERGY OF MONOLAYER GRAPHENE

Table I compares the atomization energies of monolayer graphene predicted by density functional theory (DFT) with different functionals and by diffusion quantum Monte Carlo (DMC). Our DFT static-nucleus atomization energies were obtained using the local density approximation (LDA) and Perdew–Burke–Ernzerhof (PBE) functionals with both ultrasoft [1] and Dirac–Fock pseudopotentials [2] using a plane-wave cutoff energy of 220 Ry. We compare our results with previous results in the literature [6, 7]. Both DFT-PBE and DFT-LDA calculations overestimate the atomization energy, but the error in the LDA result is significantly larger.

TABLE I: Static-nucleus atomization energy $E_{\rm atom}$ of monolayer graphene obtained in various DFT and DMC studies. The bond lengths quoted in the table are the ones used in the calculations, not necessarily the optimized bond length for the given method.

| Method | Pseudopotential | Bond length (Å) | $E_{\rm atom}$ (eV/atom) |
|---|---|---|---|
| DFT-LDA [8] | | 1.412 | 8.96 |
| DFT-LDA [6] | | 1.420 | 8.873 |
| DFT-LDA (pres. wk.) | Ultrasoft [1] | 1.420 | 8.632 |
| DFT-LDA (pres. wk.) | Dirac–Fock [2] | 1.420 | 8.578 |
| DFT-PBE [7] | Norm-conserving [9] | 1.440 | 7.847 |
| DFT-PBE [8] | | 1.424 | 7.93 |
| DFT-PBE [10] | Dirac–Fock [11] | 1.421 | 7.906 |
| DFT-PBE (pres. wk.) | Ultrasoft [1] | 1.420 | 7.873 |
| DFT-PBE (pres. wk.) | Dirac–Fock [2] | 1.420 | 7.837 |
| DMC [10] | Dirac–Fock [11] | 1.421 | 7.464(10) |
| DMC (pres. wk.) | Dirac–Fock [2] | 1.420 | 7.395(3) |

The DFT results in Table I show that using different pseudopotentials changes the calculated atomization energy of graphene by 40–70 meV/atom, which is very large on the scale of the binding energy (BE) of graphite. However, DFT-LDA and DFT-D calculations at different layer separations show that both ultrasoft and Dirac–Fock pseudopotentials give the same value for the BE of AB-stacked bilayer graphene (BLG): see Table II. The cancellation of pseudopotential errors between bilayer and monolayer graphene is much larger than between monolayer graphene and an isolated C atom, so our calculation of the BE of BLG is expected to be significantly more accurate than our calculation of the atomization energy of graphene. It should be noted that pseudopotential errors are at least as bad in DMC calculations as in DFT; although DMC is a highly accurate method, it cannot do better than permitted by the pseudopotentials used to model atoms.

## II. FINITE-POPULATION ERRORS IN OUR DIFFUSION MONTE CARLO DATA

We have carried out calculations to investigate finite-population errors [12] in our DMC calculations. Figures 1(a) and 1(b) show the non-twist-averaged DMC ground-state energy per atom for a $3 \times 3$ supercell of monolayer graphene and the DMC energy of an isolated, spin-polarized C atom against the reciprocal of the target configuration population. The DMC energies have been extrapolated linearly to zero time step in each case. The function fitted to the DMC data in Fig. 1 is $E(N_{\rm pop}) = E(\infty) + B/N_{\rm pop}$, where $N_{\rm pop}$ is the target configuration population [12]. For our Slater–Jastrow trial wave function, we find that $B = 1.4(6)$ eV for monolayer graphene in a $3 \times 3$ supercell. The gradient $B$ is of marginal significance. For populations in excess of 512 configurations the expected bias in the DMC energy is less than 2.7(12) meV/atom. We used target populations of 1024 configurations in our production calculations for supercells of $3 \times 3$ primitive cells and target populations of 512 configurations for larger supercells. Population-control biases are always positive and must largely cancel out of the BE of BLG. For an isolated C atom,

TABLE II: Comparison of DFT and DFT-D BEs of AB-stacked BLG at equilibrium separation 3.384 Å using ultrasoft and Dirac–Fock pseudopotentials.

| Method | Pseudopotential | BE (meV/atom) |
|---|---|---|
| DFT-PBE | Dirac–Fock [2] | 6.03 |
| DFT-PBE | Ultrasoft [1] | 4.87 |
| DFT-LDA | Dirac–Fock [2] | 12.39 |
| DFT-LDA | Ultrasoft [1] | 13.53 |
| DFT-D (TS) [3] | Dirac–Fock [2] | 38.35 |
| DFT-D (TS) [3] | Ultrasoft [1] | 38.22 |
| DFT-D (OBS) [4] | Dirac–Fock [2] | 59.32 |
| DFT-D (OBS) [4] | Ultrasoft [1] | 59.58 |
| DFT-D (Grimme) [5] | Dirac–Fock [2] | 27.01 |
| DFT-D (Grimme) [5] | Ultrasoft [1] | 26.57 |

the value of $B$ is not statistically significant. We have used a target population of 1024 configurations in our calculation for the C atom; the resulting population-control bias in the DMC energy is less than 1 meV.

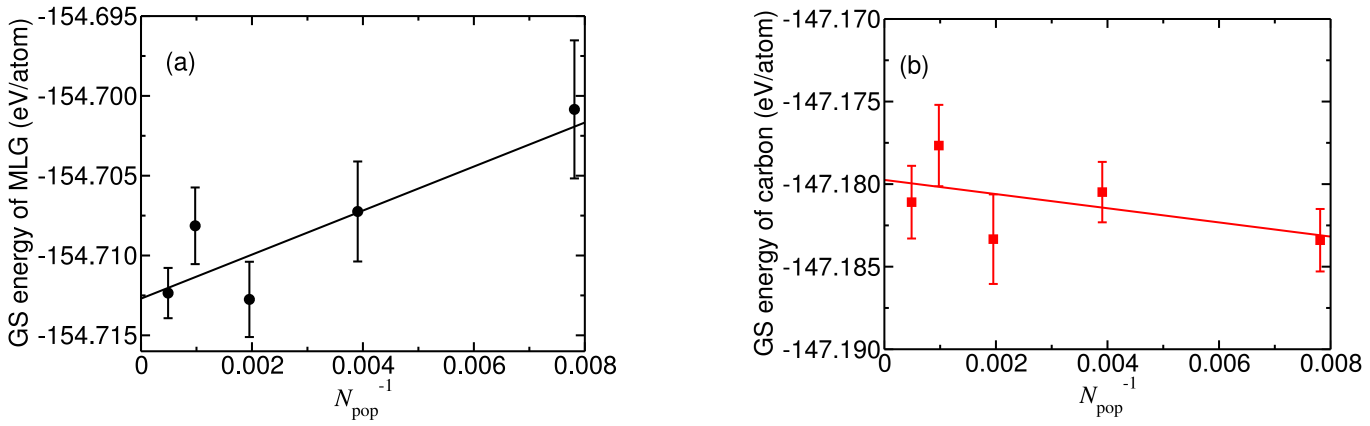


FIG. 1: (a) Non-twist-averaged DMC ground-state (GS) energy of a $3 \times 3$ cell of monolayer graphene and (b) DMC GS energy of a C atom as a function of the reciprocal of the configuration population $N_{\rm pop}^{-1}$.

## III. TIME-STEP ERRORS IN OUR DIFFUSION MONTE CARLO DATA

Figure 2(a) shows the non-twist-averaged ground-state DMC energies of $3 \times 3$ supercells of monolayer graphene and AB-stacked BLG as a function of time step. Linear extrapolations to zero time step using time steps of 0.01 and 0.04 a.u. are shown by dashed lines. The differences between the results of linear extrapolation using the time steps 0.01 and 0.04 a.u. and those obtained using three time steps 0.001, 0.005, and 0.01 a.u. are 11(3) and 13(3) meV/atom for the bilayer and monolayer, respectively. These differences indicate the magnitude of the error in the atomization energy due to residual time-step bias.

Figure 2(b) shows the non-twist-averaged DMC BE of a $3 \times 3$ cell of AB-stacked BLG against time step. Unlike the total energy, the BE varies linearly with time step across the range time steps considered. The difference between the extrapolated BE using time steps of 0.01 and 0.04 a.u. and that extrapolated using all the time steps shown in Fig. 2(b) is 1(2) meV/atom, which is negligible. Time-step bias largely cancels between the bilayer and monolayer energies, and the remaining bias in the BE may easily be removed by linear extrapolation to zero time step.

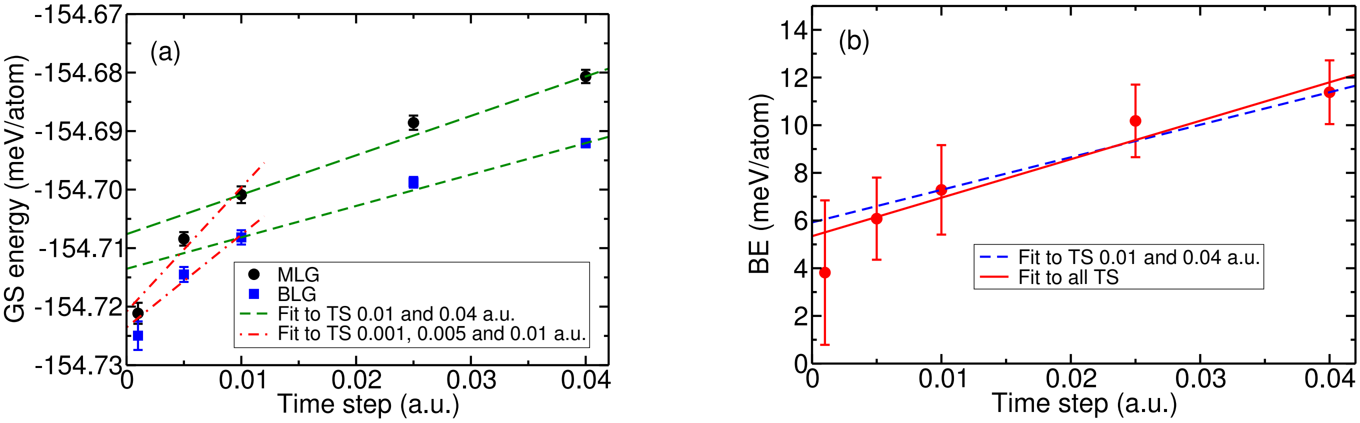


FIG. 2: (a) Non-twist-averaged DMC energy of a $3 \times 3$ cell of monolayer graphene (MLG) and AB-stacked BLG as a function of time step (TS). (b) Non-twist-averaged DMC BE of a $3 \times 3$ cell of AB-stacked BLG against time step.

## IV. CHOICE OF FITTING FUNCTION FOR THE BINDING-ENERGY CURVE

We have investigated different fitting functions for our DMC BE data for AB-stacked BLG. In Fig. 3 we compare the following fits to the DMC BE:

**Fit 1a** The maroon long-dashed line shows a fit of

$$E_{\text{bind}}(d) = a + b(d - d_0)^2 + c(d - d_0)^3 \tag{1}$$

to the DMC BE data at interlayer separations $d = 2.8$, 3.384, and 3.84 Å, where $a$, $b$, and $c$ are fitting parameters and $d_0 = 3.384$ Å is fixed at the vdW-DF interlayer equilibrium separation [13].

**Fit 1b** The red short-dashed line shows a fit of Eq. (1) to the DMC BE data at interlayer separations $d = 2.6$, 2.8, 3.384, and 3.84 Å. This time $a$, $b$, $c$, and $d_0$ are all fitting parameters.

**Fit 1c** The green dot-dashed line shows a fit of Eq. (1) to the DMC BE data at interlayer separations $d = 2.8$, 3.384, 3.84, and 4.3 Å. Again, $a$, $b$, $c$, and $d_0$ are all fitting parameters.

**Fit 1d** The blue dash-double dotted line shows a fit of Eq. (1) to all our DMC BE data. Again, $a$, $b$, $c$, and $d_0$ are all fitting parameters.

**Fit 2** The solid black line shows a fit of

$$E_{\text{bind}}(d) = \alpha \exp(-\beta d) + \gamma d^{-4} \tag{2}$$

to all our DMC BE data, where $\alpha$, $\beta$, and $\gamma$ are fitting parameters [14].

**Fit 3** The solid magenta line shows a fit of

$$E_{\text{bind}}(d) = A_4 d^{-4} + A_8 d^{-8} + A_{12} d^{-12} + A_{16} d^{-16} \tag{3}$$

to all our DMC BE data, where the $\{A_i\}$ are fitting parameters.

Equation (3) has the correct $d^{-4}$ form of decay for the BE at intermediate range and has a reasonable model of the hard-core repulsion. The $\chi^2$ values obtained with Fits 2 and 3 are 1.3 and 0.007 per data point, respectively, compared with 0.4 per data point for Fit 1d, which has the same number of fitting parameters as Fit 3. The $\chi^2$ value per data point for Fits 1a–1c is zero, because the number of data points is equal to the number of parameters. Fit 2 shows unphysical behavior: the exponential term prefers to be attractive while the $d^{-4}$ tries to be repulsive. We have therefore used Fit 3 to obtain the breathing-mode frequency presented in the main body of our article.

In Table III we compare the equilibrium separation $d_0$, the corresponding BE $E_{\text{bind}}(d_0)$, the curvature $E''_{\text{bind}}(d_0)$, and the out-of-plane optical phonon frequency (the breathing mode ZO′) obtained with the different fits to our DMC BE data.

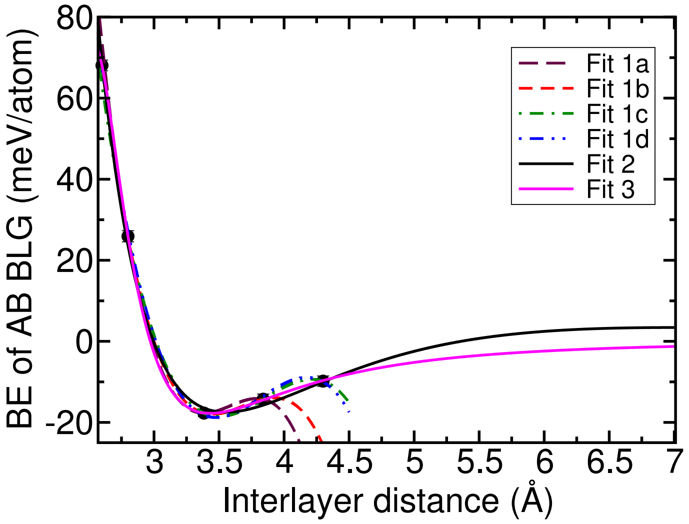


FIG. 3: DMC BE of AB-stacked BLG against interlayer separation using different fitting curves.

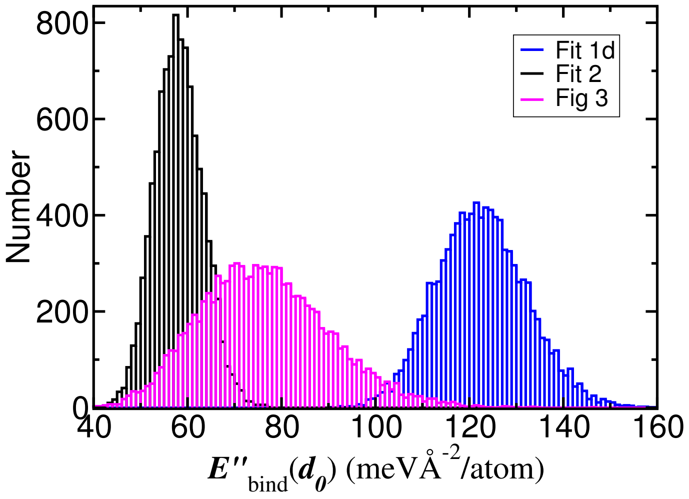


FIG. 4: Histogram of $E''_{\rm bind}(d_0)$ obtained in bootstrap Monte Carlo sampling of Fits 1d, 2, and 3 with 10,000 samples.

To evaluate error bars on quantities such as the second derivative of the BE at the minimum and the corresponding phonon frequency, we used bootstrap Monte Carlo sampling of our data together with repeated $\chi^2$ fits. In Fig. 4, histograms of $E''_{\rm bind}(d_0)$ for Fits 1d, 2 and 3 are shown. The phonon frequencies obtained using Fits 2 and 3 are in good agreement, although the difference between Fits 1d and 3 is more significant. However, we believe Fit 3 to be more reliable because it is constructed to have the correct asymptotic behavior.

[1] S.J. Clark *et al.*, Z. Kristallogr. **220**, 567 (2005).
[2] J.R. Trail and R.J. Needs, J. Chem. Phys. **122**, 014112 (2005).
[3] A. Tkatchenko and M. Scheffler, Phys. Rev. Lett. **102**, 073005 (2009).
[4] F. Ortmann, F. Bechstedt, and W.G. Schmidt, Phys. Rev. B **73**, 205101 (2006).
[5] S. Grimme, J. Comput. Chem. **27**, 1787, (2006).
[6] M. Hasegawa and K. Nishidate, Phys. Rev. B **70**, 205431 (2004).
[7] A. Hansson, F. de Brito Mota, and R. Rivelino, Phys. Rev. B **86**, 195416 (2012).
[8] G. Graziano *et al.*, J. Phys.: Condens. Matter **24**, 424216 (2012).
[9] N. Troullier and J.L. Martins, Phys. Rev. B **43**, 1993 (1991).

TABLE III: Equilibrium separation $d_0$ and corresponding BE $E_{\rm bind}(d_0)$, second derivative of the BE at the minimum $E''_{\rm bind}(d_0)$, and out-of-plane phonon frequency $\omega_{\rm ZO'}$ that are obtained by fitting different curves to our DMC data for the BE of BLG. Experimental results [15] are shown for comparison.

| Fit | $d_0$ (Å) | $E_{\rm bind}(d_0)$ (meV/atom) | $E''_{\rm bind}(d_0)$ (meV Å$^{-2}$/atom) | $\omega_{\rm ZO'}$ (cm$^{-1}$) |
|---|---|---|---|---|
| Fit 1a | 3.384 | −17.7(9) | 131(11) | 109(4) |
| Fit 1b | 3.45(4) | −18(1) | 110(17) | 100(8) |
| Fit 1c | 3.50(4) | −18.6(8) | 109(12) | 99(7) |
| Fit 1d | 3.48(3) | −18.8(8) | 122(9) | 105(4) |
| Fit 2 | 3.55(2) | −17.5(7) | 58(5) | 72(3) |
| Fit 3 | 3.43(4) | −17.8(8) | 76(13) | 83(7) |
| Experiment [15] | | | 70(4) | 80(2) |
| Experiment [16] | | | 89 | 89 |


[10] H. Shin *et al.*, J. Chem. Phys. **140**, 114702 (2014).
[11] M. Burkatzki, C. Filippi, and M. Dolg, J. Chem. Phys. **126**, 234105 (2007).
[12] C.J. Umrigar, M.P. Nightingale, and K.J. Runge, J. Chem. Phys. **99**, 2865 (1993).
[13] I. Brihuega *et al.*, Phys. Rev. Lett. **109**, 196802 (2012).
[14] L. Spanu *et al.*, Phys. Rev. Lett. **103**, 196401 (2009).
[15] C.H. Lui and T.F. Heinz, Phys. Rev. B **87**, 121404(R) (2013).
[16] S. Milana, D. Yoon, M. Ijäs, W. P. Han, P.H. Tan,N.M. Pugno, T. Bjorkman, A. Krashenninnikov, and A.C. Ferrari, Determination of Shear Modulus and Out of Plane Young's Modulus of Layered Materials by Raman spectroscopy, Graphene Week, 2015.
